# Supplementary material for: Mechanical stress dependence of the Fermi level pinning on an oxidized silicon surface
Source: arXiv:1810.11219 source file (2019-02-04)
Supplement: Supplementary file 1 [file Supplementary_Material.pdf]

**Supplementary Material**

H. Li et al., "Mechanical stress dependence of the (001) surface band bending on natively-oxidized silicon"

1. Sample preparation

Simple macroscopic silicon cantilevers are fabricated from a (001) oriented silicon-on-insulator (SOI) wafer [p-type doped (boron, $\rho < 0.01$ Ωcm), with a 5 μm thick device layer, a 1 μm thick buried oxide layer and a $d = 400$ μm thick handle] as follows. First the device layer oxide is removed using a dilute (5 %) hydrofluoric acid solution, following which a 50 nm thick layer of platinum is thermally evaporated onto the device layer via a shadow mask. During evaporation the surface is exposed to a low energy argon plasma, after which ohmic contacts are formed by annealing (600°C for 1 minute under a forming gas, 95 % $N_2$/ 5 % $H_2$, atmosphere). A diamond saw is then used to cut $l = 11$ mm long, $b = 3$ mm wide cantilevers from the SOI where the long axis is parallel to the $\langle 110 \rangle$ crystal direction. The cantilevers, which are protected during this procedure with a 1 μm thick photoresist (AZ1518) layer, are cut so that the ohmic contacts are present at each end of the cantilever as shown in Fig. 1(a). Following dicing the cantilevers were stored with the photoresist in place for two months. Two weeks prior to the experiments reported here, the photoresist was removed with a stripper (SVC-14), rinsed in acetone, iso-propyl alcohol and de-ionized water before drying with nitrogen. During this time the device layer formed a native oxide in the ambient atmosphere (25 °C, 45 % r.h.).

2. Oxide thickness results in energy shift

Since the "chemical shift" of oxidation states is surface oxide thickness dependence[1], i.e. the differences between silicon oxidation states 2p core-level and bulk silicon 2p core-level increase with increasing oxide thickness. Therefore, in addition to stress, the inhomogeneous oxide thickness can also shift the observed bulk Si 2p core-level and discrimination of the origin of the peak shift is therefore *a priori* difficult. For example, the absolute kinetic energy difference between $Si^{4+}$ 2p core-level and Si 2p core-level versus oxide thickness in $x$-direction is plotted in Fig. 1 (red dots). In $x$-direction, the cantilever has less influence from stress due to the homogeneous stress distribution, however the more influence from oxide thickness due to the variation of $SiO_2$ thickness across the width. The value of energy shift of $Si^{4+}$ approximates to that without stress reported by *Th. Eickhoff*, (see empty circles of Si 2p in Fig. 1), the slope respects to oxide thickness is about 50 meV/Å$^2$.

| | Area in Fig. 2 | Intensity ($/10^5$) | Kinetic energy shift from Si 2p 3/2 (eV) | Width (eV) |
|---|---|---|---|---|
| **$Si^0$ 2p 3/2** | B | 17.5 | 0 | 0.44 |
| **Si 2p 2nd plane** | I | 4 | -0.3 | 0.37 |
| **$Si^{1+}$ 2p 3/2** | 1+ | 2.5 | -0.9 | 0.57 |
| **$Si^{2+}$ 2p 3/2** | 2+ | 1.6 | -1.88 | 0.9 |
| **$Si^{3+}$ 2p 3/2** | 3+ | 5.6 | -2.9 | 1.1 |
| **$Si^{4+}$ 2p 3/2** | 4+ | 16.2 | -4.1 | 1.66 |

**Table 1:** The fitting parameters used in Fig. 2.

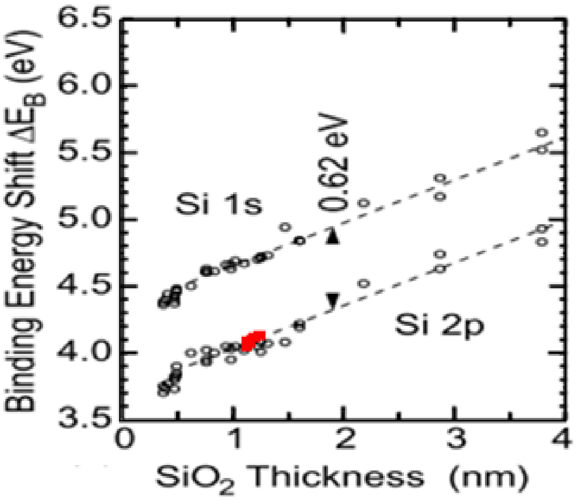


Figure 1: Energy shift of $Si^{4+}$ versus oxide thickness from $x$-direction of cantilever under tensile stress (red dots) and reported by *Th. Eickhoff* (empty circles of Si 2p) respectively[2].

This energy shift of $Si^{4+}$ induced by oxide thickness then consequently influences binding energy of bulk Si 2p core-level, therefore it is important to separate the stress effect from oxidation effect to clearly estimate the band bending energy shift induced by stress. It is possible to estimate the surface silicon oxide thickness, $d_{\mathrm{ox}}$, from the relative integrated intensities of the bulk and oxide XPS components according to

$$d_{\mathrm{ox}} = \lambda_f \sin\theta \, ln\left[\frac{I_{SiO_2}}{I_{Si}} A + 1\right], \quad (1)$$

where $A = D_s\lambda_s/D_f\lambda_f$. Here $\theta = 90°$ is the take-off angle related to the experimental geometry, $D_s$ and $D_f$ are the densities of silicon atoms in the crystal and surface oxide layer respectively, and $\lambda_s =$ 0.56 nm and $\lambda_f = 0.54$ nm are the electron escape depths for this photon wavelength[3,4]. Using the values in Table 1 corresponding to the spectrum shown in the top panel of Fig. 2 this yields an approximate oxide thickness of 1.15 nm for the pixel shown in black in the bottom panel of Fig. 2. By repeating this procedure for each spectrum measured by scanning the sample in front of the beam, a map of the $SiO_2$ thickness is obtained as shown in Fig. 2 (bottom panel). Intriguingly, the silicon oxide is systematically thinner along the central axis of the cantilever than along its two edges. This is attributed to the fact that during the 2-month storage time mentioned above, the protective photoresist only allows for oxidation of the silicon to occur via oxygen diffusion from the sawn edges of the cantilever. The effective oxygen exposure time is therefore longest towards the edges of the cantilever, resulting in an oxide layer that tends to be thicker there than along the middle of the cantilever. This is also apparent in the cut shown in Fig. 3(a) where the inverse proportionality between oxide thickness and XPS peak intensity is explicitly clear (see also Fig. 3(b)).

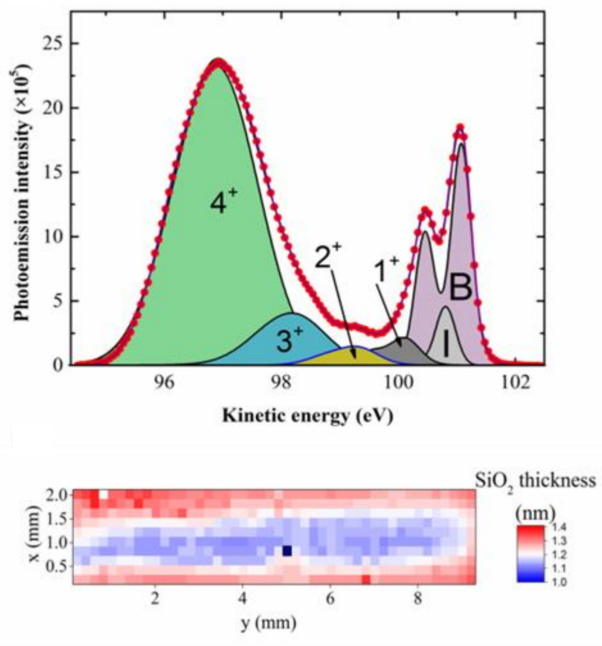


Figure 2: (top) An example Si 2p core level XPS spectrum at the surface of a cantilever. The red dots present measured spectrum while the black curve presents the fitting result. Each state component is presented by a colored area and the fitting parameters are presented in Table 1. (bottom) A map of the estimated silicon oxide thickness based on the fitting procedure (see text). The black rectangle represents the pixel corresponding to the spectrum shown in the top panel.

The correction for the variable oxide thickness is achieved by extracting (for each value of the coordinate x) only pixels whose oxide thickness is the same along the y-direction, at least to within an arbitrarily imposed 2 % variation around some mean value. It's then possible, to estimate the unique stress induced changes in Si 2p core-levels. In order to avoid as much as possible the influence of the oxide related peaks, we focus on the bulk Si 2p core-level peak position for the study of stress-induced core-level shifts since this peak is furthest from the oxide related peaks. Most importantly the pixels used to consider the stress induced changes in bulk Si 2p core-level should have identical oxide thickness and the thickness-intensity relationship shown in Fig. 3 can then be used to select similar intensity pixels from XPS maps as shown in Fig. 4.

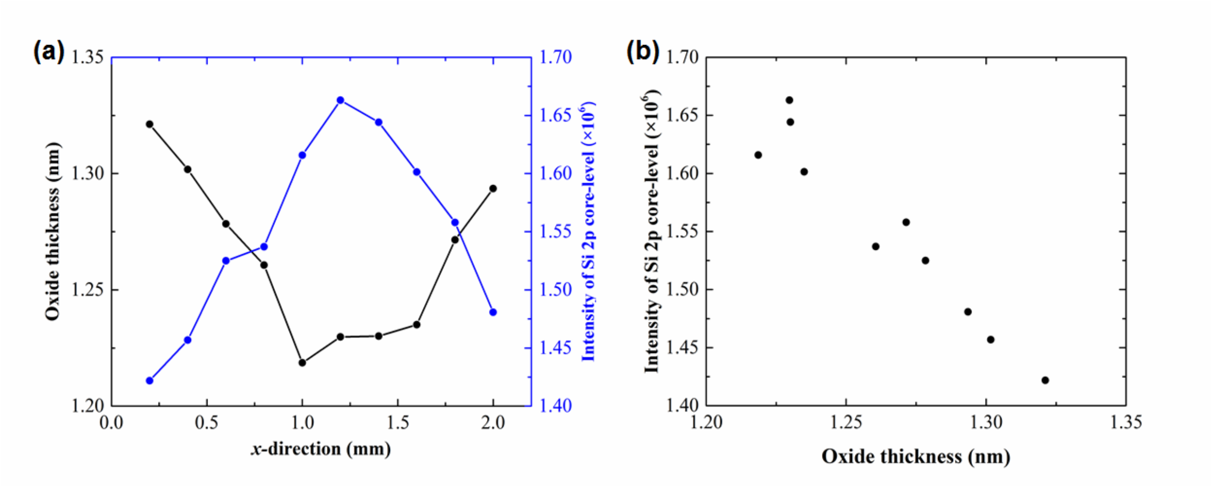


Figure 3: (a) The oxide thickness (black curve) and the intensity of Si 2p core-level (blue curve) versus x-direction position on the cantilever respectively. (b) Intensity of Si 2p core-level is linear to the oxide thickness indicates that the thicker oxide layer corresponds to lower intensity, *vice versa*.

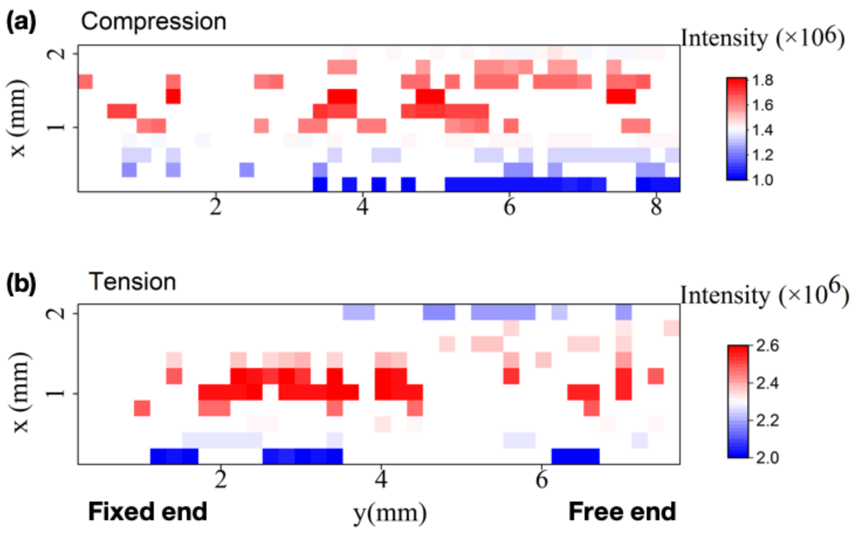


Figure 4: To avoid the influences of oxide effect to energy shift, the pixels with similar intensity along each $y$-direction are selected and presented under (a) tensile and (b) compressive stress.

3. Determination of XPS peak positions with meV accuracy

In order to illustrate the ability to resolve XPS peaks with meV accuracy, 3 example spectra are chosen (corresponding to the pixels shown in Fig. 5(a)) for the cantilever whose top surface is under tensile stress. These spectra are normalized in order to more easily observe the peak position shifts in Fig. 5(b). The colors of the lines and data points in Fig. 5(b) correspond to the equivalently colored pixels in Fig. 5(a) whose $x$-coordinate is identical.

Since the sensitivity of each pixel in electron detector is not absolutely equal, the observed spectrum would be somehow consequently affected by this factor. From the inset of Fig. 5(b), the zoomed black

rectangle area of the bulk Si 2p core-level in Fig. 5(b), the spectra are not perfectly smooth due to varied sensitivity of detector. Despite the influence of sensitivity, the kinetic energy peak position is still clearly visible that leftward shifts from red spectrum (with no stress) to the black spectrum (with maximum stress). The gray column presents 20 meV range in the figure, which is approximate to the scale of stress induced changes in the energy in our case. The energy between 2 raw data points in the spectrum is 10.4 meV, the stress is then able to shift energy of approximate 3 data points distance of spectrum. Fitting procedure allows us to precisely estimate the Si 2p core-level of bulk silicon and its different oxidation states, in this case, the shape and width of these components are fixed, the only free parameters can play with are the intensity and peak position. From the fitting result, the 95% confidence interval of each parameter can be obtained; the standard error of bulk Si 2p core-level peak position can be consequently calculated by using 95% confidence interval which is about 3meV.

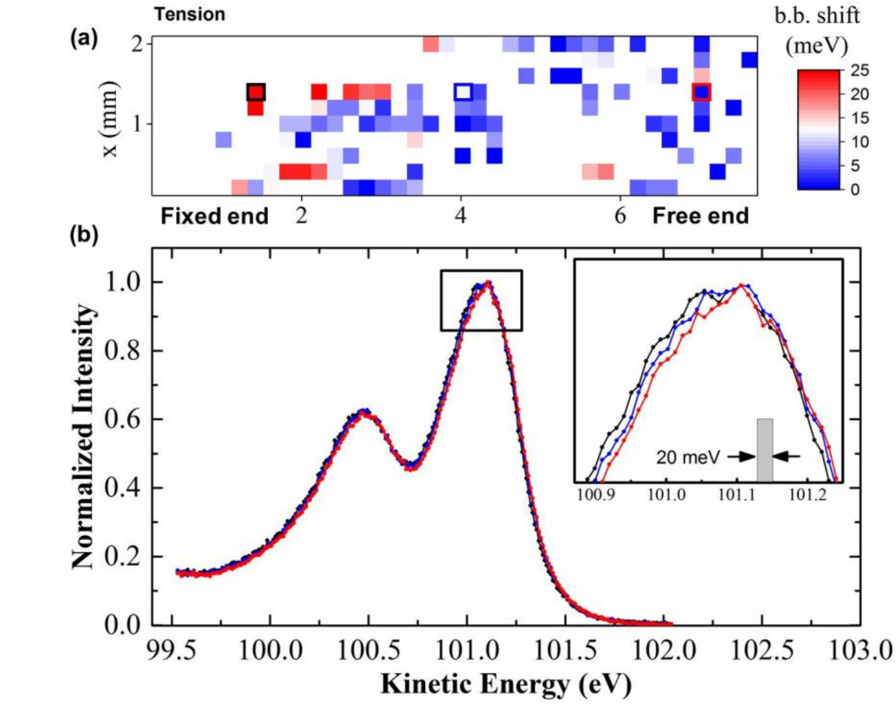


Figure 5: (a) The surface band bending shift of tensile stressed cantilever, 3 selected pixels are presented by colored rectangles, their XPS spectra are shown in (b). The stress is indicated by position on the cantilever, stress induced changes in Si-2p core level can be seen by peak position shift.

The same is also true for compression, 3 XPS spectra have been selected in Fig. 6 (a) for the cantilever whose top surface is under compressive stress. The peak position of kinetic energy under compressive stress is also leftward shift from red spectrum (with no stress) to the black spectrum (with maximum stress) as shown in Fig. 6(b).

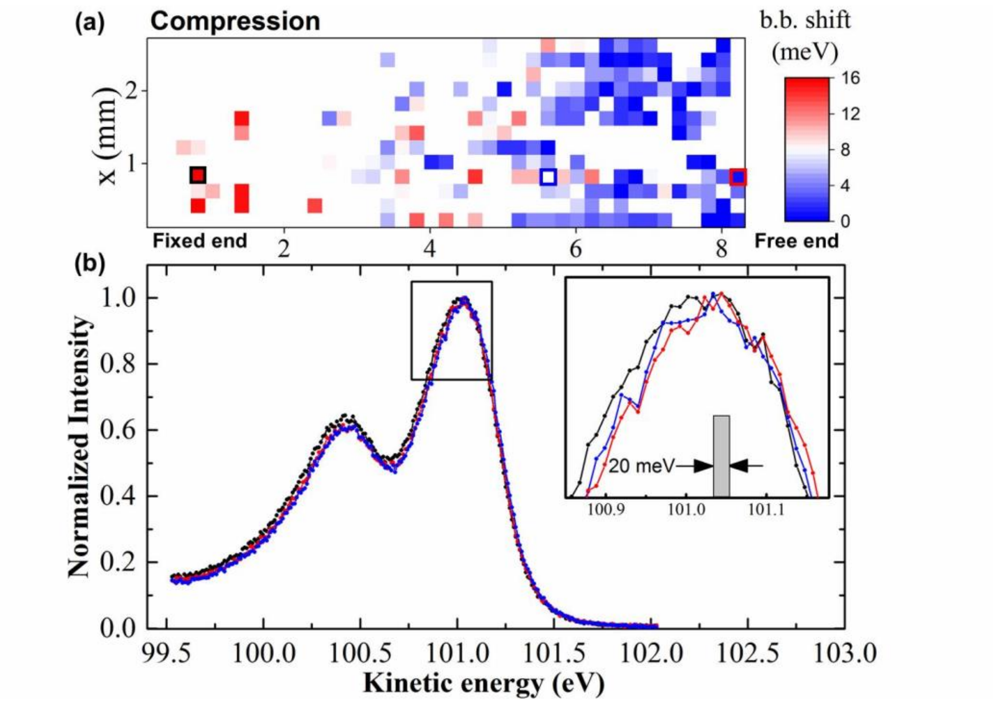


Figure 6: (a) The surface band bending shift of compressive stressed cantilever, 3 selected pixels are presented by colored rectangles, their XPS spectra are shown in (b). The stress is indicated by position on the cantilever, stress induced changes in Si-2p core level can be seen by peak position shift.

---

[1] T. Eickhoff, V. Medicherla & W. Drube *Final state contribution to the Si 2p binding energy shift in SiO2/Si(1 0 0) J. Electron Spectros. Relat. Phenomena* **137–140**, 85 (2004).

[2] I. Jiménez and J.L. Sacedón *Influence of Si oxidation methods on the distribution of suboxides at Si/SiO2 interfaces and their band alignment: A synchrotron photoemission study*, Surf. Sci. **482**–**485**, 272 (2001).

[3] A. Jablonski and C. Powell. *Relationships between electron inelastic mean free paths, effective attenuation lengths, and mean escape depths* J. Electron Spectros. Relat. Phenomena **100**, 137 (1999).

[4] M.P. Seah and W.A. Dench. *Quantitative Electron Spectroscopy of Surfaces: A Standard Data Base for Electron Inelastic Mean Free Paths in Solids* Surf. Interface Anal. **1**, 2 (1979).
